# Supplementary material for: Cardiac Mechano-Electrical Dynamical Instability
Source: arXiv:1908.05144 ancillary file (2019-08-14)
Supplement: Supplementary file 1 [file SI.pdf]

# Supplemental Material
# Cardiac Mechano-Electrical Dynamical Instability

L. D. Weise[1,2] and A. V. Panfilov[1]

[1]*Department of Physics and Astronomy, Ghent University, Krijgslaan 281, S9, Ghent, 9000, Belgium*

[2]*Department of Theoretical Biology, Utrecht University, Padualaan 8, Utrecht, 3584 CH, The Netherlands*

# Table of Contents


| section | pages | title |
|---|---|---|
| A | 3 | Illustration of MEDI in 2D setup (Figure 1 in paper): observables along diagonal |
| B | 4 | APD(DI): dynamical restitution *vs* wave front-back collision |
| C | 5 | Supplementary video captions |

## Illustration of MEDI in 2D setup (Figure 1 in paper): observables along diagonal

We showed in Figure 1 in the paper that MEDI manifests itself as a local wave by wave increase in APD while DI decreases. Here we use the same simulation used for Figure 1 in the paper to illustrate how the transmembrane potential and availability of sodium channels are affected by wave front-back collision. We show the results in Figure 1. From the top

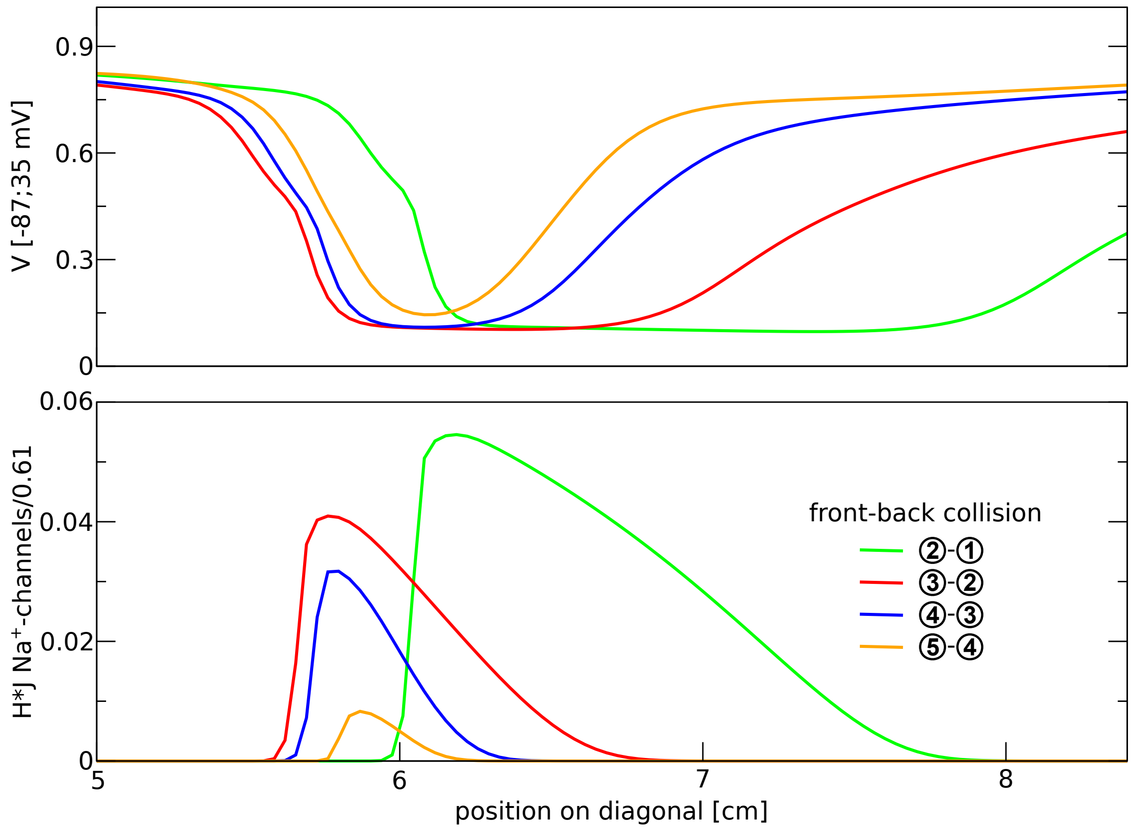


FIG. 1: Mechanism of MEDI dynamical instability. Simulation used for Figure 1 in the paper. Periodical wave initiation in left, upper corner: ten waves were initiated with period 340 $ms$, then seven waves with period 300 $ms$. Observables transmembrane voltage (top) and availability of sodium channels (bottom) were measured along the diagonal (from upper, left to lower, right corner) for last five wave-front collisions leading to wave break are shown. Snapshots are taken at the moments of front-back collision (when DI is minimal) at simulation times $[ms]$: $280; 570; 870; 1190$. Side length of model 15 $cm$. $G_s = 50\ S/F$.

panel we can see that the colliding waves start their action potential from an increasingly depolarized state. The sodium channels are affected by the transmembrane voltage. And in fact we see from the lower panel that the availability of sodium channels decreases from wave to wave at the collision position. This result is connected to our finding shown in Figure 4B in the paper: shorter DI due to wave front-back collision causes the inactivation of sodium channels.

We can conclude that the constantly stretched fiber setup used to explain the mechanism in more detail, resembles MEDI in the full 2D setup.

## APD(DI): dynamical restitution *vs* wave front-back collision

Here we show APD as a function of DI in a dynamical restitution protocol and during wave front-back collision. We used the following dynamical restitution protocol “shrinking circle experiment. We initiated an unidirectionally propagating wave in a circular, constantly stretched fiber ($I_{sac} = G_s(V - E_s)$). We gradually decreased the circumference of the circular fiber, and measured APD and DI. In Figure 2 we show APD as a function of DI for both, the collision experiment, and the dynamic restitution protocol (both for $Gs = 10.5\ S/F$). Note

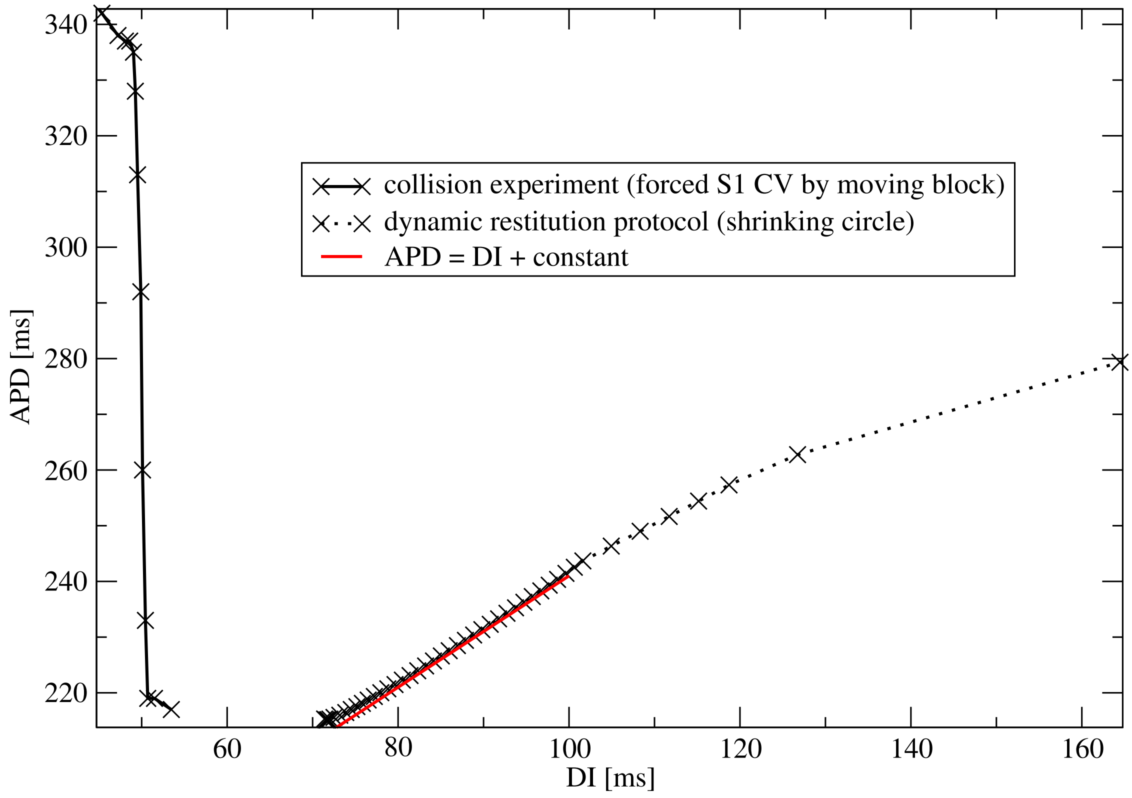


FIG. 2: APD as function of DI in collision experiment (compare Figure 3) and dynamical restitution experiment (shrinking circle). Circumference of the circle is decreased by 2.5 $mm$ after every 10 rotations of the wave and APD and DI is measured. $Gs = 10.5\ S/F$.

that the restitution curve (dotted line) is monotonically increasing, a longer DI causes a longer APD. Interestingly, we see that for $DI < 100\ ms$ the slope of the restitution curve is close to the slope of 1 (compare red line) - the theoretical predictor for the onset of alternans. Break happened via alternans at a DI of $\approx 70\ ms$.

The APD(DI) behavior in the collision experiment (connected line) is substantially different from the APD restitution curve. For wave front-back collisions causing a $DI < 55\ ms$ we see that a decrease in DI (stronger collision) causes a steep increase of APD.

We can conclude that APD(DI) behaviour during wave front-back collision can not be explained with classical restitution theory.

## Supplementary video captions

**Illustration of MEDI**
**(compare Figure 1 in paper)**

**Supplementary Video 1**. Simulation used for Figure 1 in paper. Periodical wave initiation in left, upper corner: ten waves were initiated with period 340 *ms*, then seven waves with period 300 *ms*. Seven last waves are shown. Time is shifted, so that 0 *ms* is when wave front ② collides with wave back ① (consistent with Figure 1 in paper). Observables transmembrane voltage, intracellular calcium concentration, local deformation and availability of sodium channels are shown in deforming 2D system. Side length of model 15 *cm*. $G_s = 50\ S/F$.
**Supplementary Video 2**. Simulation used for Figure 1 in paper. Periodical wave initiation in left, upper corner: ten waves were initiated with period 340 *ms*, then seven waves with period 300 *ms*. Seven last waves are shown. Time is shifted, so that 0 *ms* is when wave front② collides with wave back ① (consistent with Figure 1 in paper). Observables transmembrane voltage, local deformation and availability of sodium channels along diagonal line (upper, left corner to lower, right corner) a line (0.25 *cm* from are shown. Side length of model 15 *cm*. $G_s = 50\ S/F$.

**Illustration of rapid spiral wave meandering caused by MEDI**
**(compare Figure 5 in paper)**

Simulation used for Figure 5 in paper. Spiral was initiated in the medium without MEF ($G_s = 0\ S/F$), let rotate for 2 *s*, then system was saved and used as starting point for simulations with MEF. Time starts when $I_{sac}$ is activated. Side length of model 12.5 *cm*.
**Supplementary Video 3**. $G_s = 12.5\ S/F$.
**Supplementary Video 4**. $G_s = 25.0\ S/F$.
**Supplementary Video 5**. $G_s = 37.5\ S/F$.
**Supplementary Video 6**. $G_s = 50.0\ S/F$.
**Supplementary Video 7**. $G_s = 62.5\ S/F$.
